# Supplementary material for: Enhanced production of $\Lambda_{b}^{0}$ baryons in high-multiplicity $pp$ collisions at $\sqrt{s} = 13$ TeV
Source: arXiv:2310.12278 source file (2024-02-22)
Supplement: Supplementary file 1 [file supplementary.tex]

\clearpage
\FloatBarrier
\section*{Appendix: Supplemental material}
\label{sec:Supplementary}  

The ratio of $\Lb$ to $\Bd$ cross-sections $\sigma_{\Lb}/\sigma_{\Bd}$ as a function of $\pt$ and normalized multiplicity $\Nvelo / \langle \Nvelo \rangle$$_{\mathrm{NB}}$ are given in Tables \ref{tab:tab1} and \ref{tab:tab2}, respectively.  Tables \ref{tab:tab3}, \ref{tab:tab4}, and \ref{tab:tab5} give the ratio versus the total VELO multiplicity for low-, intermediate-, and high-multiplicity ranges, respectively. Tables \ref{tab:tab6}, \ref{tab:tab7}, and \ref{tab:tab8} provide the ratio versus the backward multiplicity metric for low-, intermediate-, and high-multiplicity ranges, respectively.

\begin{table}[h]
\centering
\begin{tabular}{cc}
$\pt$ range [GeV/$c$] & $\sigma_{\Lb}/\sigma_{\Bd}$ \\

\midrule
0 -- 2 & $0.45\pm0.03$ \\
2 -- 4 & $0.44\pm0.02$ \\ 
4 -- 6 & $0.46\pm0.02$ \\ 
6 -- 8 & $0.41\pm0.02$ \\ 
\hspace{0.2cm}8 -- 10 & $0.39\pm0.02$ \\ 
10 -- 12 & $0.33\pm0.01$ \\ 
12 -- 14 & $0.29\pm0.01$ \\ 
14 -- 16 & $0.27\pm0.01$ \\ 
16 -- 18 & $0.23\pm0.01$ \\ 
18 -- 20 & $0.21\pm0.01$ \\ 
20 -- 22 & $0.21\pm0.02$ \\ 
22 -- 24 & $0.23\pm0.02$ \\ 
24 -- 26 & $0.19\pm0.02$ \\ 
26 -- 28 & $0.18\pm0.03$ \\ 
28 -- 30 & $0.16\pm0.03$ \\ 
\end{tabular}
\caption{Ratio of cross-sections as a function of $\pt$, as shown in Fig. \ref{fig:Fig1}. The additional $^{+19\%}_{-16\%}$ global uncertainty due to the uncertainty in the branching fractions is not included.}
\label{tab:tab1}
\end{table}

\begin{table}[h]
\centering
\begin{tabular}{cc}
\Nvelo/$\langle \Nvelo \rangle$$_{\mathrm{NB}}$ & $\sigma_{\Lb}/\sigma_{\Bd}$ \\
\midrule
0.13 -- 0.40 &  $0.25\pm0.05$ \\
0.40 -- 0.53 &  $0.35\pm0.03$ \\
0.53 -- 0.66 &  $0.36\pm0.03$ \\
0.66 -- 0.79 &  $0.38\pm0.02$ \\
0.79 -- 1.06 &  $0.42\pm0.02$ \\
1.06 -- 1.32 &  $0.43\pm0.02$ \\
1.32 -- 1.59 &  $0.46\pm0.03$ \\
1.59 -- 1.85 &  $0.47\pm0.03$ \\
1.85 -- 2.12 &  $0.48\pm0.03$ \\
2.12 -- 2.65 &  $0.49\pm0.03$ \\
2.65 -- 3.31 &  $0.49\pm0.03$ \\
3.31 -- 3.97 &  $0.48\pm0.03$ \\
3.97 -- 5.29 &  $0.44\pm0.03$ \\
5.29 -- 6.61 &  $0.60\pm0.08$ \\
\end{tabular}

\caption{Ratio of cross-sections as a function of multiplicity, as shown in Fig. \ref{fig:Fig3}. The additional $^{+19\%}_{-16\%}$ global uncertainty due to the uncertainty in the branching fractions is not included.}
\label{tab:tab2}    
\end{table}

\begin{table}[h]
\centering
\begin{tabular}{cc}
$\pt$ range [GeV/$c$] & $\sigma_{\Lb}/\sigma_{\Bd}$ \\
\midrule
0 -- 2 & $0.35\pm0.05$ \\
2 -- 4 & $0.41\pm0.03$ \\
4 -- 6 & $0.38\pm0.02$ \\
6 -- 8 & $0.35\pm0.02$ \\
\hspace{0.2cm}8 -- 10 & $0.29\pm0.02$ \\
10 -- 12 & $0.23\pm0.02$ \\
12 -- 14 & $0.21\pm0.02$ \\
14 -- 16 & $0.18\pm0.02$ \\
16 -- 18 & $0.12\pm0.02$ \\
18 -- 20 & $0.18\pm0.05$ \\

\end{tabular}
\caption{Ratio of cross-sections for low multiplicity data, as measured using VELO tracks, shown in blue in the left panel of Fig. \ref{fig:Fig4}. The additional $^{+19\%}_{-16\%}$ global uncertainty due to the uncertainty in the branching fractions is not included.}
\label{tab:tab3}
\end{table}

\begin{table}[h]
\centering
\begin{tabular}{cc}
$\pt$ range [GeV/$c$] & $\sigma_{\Lb}/\sigma_{\Bd}$ \\
\midrule
0 -- 2 & $0.51\pm0.04$ \\
2 -- 4 & $0.45\pm0.02$ \\
4 -- 6 & $0.46\pm0.02$ \\
6 -- 8 & $0.42\pm0.02$ \\
\hspace{0.2cm}8 -- 10 & $0.38\pm0.02$ \\
10 -- 12 & $0.33\pm0.02$ \\
12 -- 14 & $0.28\pm0.02$ \\
14 -- 16 & $0.25\pm0.02$ \\
16 -- 18 & $0.23\pm0.02$ \\
18 -- 20 & $0.17\pm0.02$ \\
20 -- 22 & $0.20\pm0.02$ \\
22 -- 24 & $0.19\pm0.02$ \\
\end{tabular}
\caption{Ratio of cross-sections for intermediate multiplicity data, as measured using VELO tracks, shown in black in the left panel of Fig. \ref{fig:Fig4}. The additional  $^{+19\%}_{-16\%}$ global uncertainty due to the uncertainty in the branching fractions is not included.}
\label{tab:tab4}
\end{table}

\begin{table}[h]
\centering
\begin{tabular}{cc}
$\pt$ range [GeV/$c$] & $\sigma_{\Lb}/\sigma_{\Bd}$ \\
\midrule
0 -- 2 & $0.49\pm0.05$ \\
2 -- 4 & $0.45\pm0.02$ \\
4 -- 6 & $0.51\pm0.02$ \\
6 -- 8 & $0.45\pm0.02$ \\
\hspace{0.2cm}8 -- 10 & $0.44\pm0.02$ \\
10 -- 12 & $0.35\pm0.02$ \\
12 -- 14 & $0.32\pm0.02$ \\
14 -- 16 & $0.30\pm0.02$ \\
16 -- 18 & $0.25\pm0.02$ \\
18 -- 20 & $0.25\pm0.02$ \\
20 -- 22 & $0.24\pm0.02$ \\
22 -- 24 & $0.22\pm0.02$ \\

\end{tabular}
\caption{Ratio of cross-sections for high multiplicity data, as measured using VELO tracks, shown in red in the left panel of Fig. \ref{fig:Fig4}. The additional $^{+19\%}_{-16\%}$ global uncertainty due to the uncertainty in the branching fractions is not included.}
\label{tab:tab5}
\end{table}

\begin{table}[h]
\centering
\begin{tabular}{cc}
$\pt$ range [GeV/$c$] & $\sigma_{\Lb}/\sigma_{\Bd}$ \\
\midrule
0 -- 2 & $0.39\pm0.04$ \\
2 -- 4 & $0.42\pm0.02$ \\
4 -- 6 & $0.42\pm0.02$ \\
6 -- 8 & $0.39\pm0.02$ \\
\hspace{0.2cm}8 -- 10 & $0.37\pm0.01$ \\
10 -- 12 & $0.29\pm0.02$ \\
12 -- 14 & $0.31\pm0.02$ \\
14 -- 16 & $0.23\pm0.02$ \\
16 -- 18 & $0.19\pm0.02$ \\
18 -- 20 & $0.19\pm0.02$ \\
20 -- 22 & $0.21\pm0.03$ \\
22 -- 24 & $0.24\pm0.03$ \\
\end{tabular}
\caption{Ratio of cross-sections for low multiplicity data, as measured using backward tracks, shown in blue in the right panel of Fig. \ref{fig:Fig4}. The additional $^{+19\%}_{-16\%}$ global uncertainty due to the uncertainty in the branching fractions is not included.}
\label{tab:tab6}
\end{table}

\begin{table}[h]
\centering
\begin{tabular}{cc}
$\pt$ range [GeV/$c$] & $\sigma_{\Lb}/\sigma_{\Bd}$ \\
\midrule
0 -- 2 & $0.41\pm0.05$ \\
2 -- 4 & $0.49\pm0.03$ \\
4 -- 6 & $0.50\pm0.02$ \\
6 -- 8 & $0.44\pm0.02$ \\
\hspace{0.2cm}8 -- 10 & $0.43\pm0.02$ \\
10 -- 12 & $0.33\pm0.02$ \\
12 -- 14 & $0.29\pm0.02$ \\
14 -- 16 & $0.27\pm0.02$ \\
16 -- 18 & $0.26\pm0.02$ \\
18 -- 20 & $0.23\pm0.02$ \\
20 -- 22 & $0.21\pm0.02$ \\
22 -- 24 & $0.18\pm0.02$ \\
\end{tabular}
\caption{Ratio of cross-sections for intermediate multiplicity data, as measured using backward tracks, shown in black in the right panel of Fig. \ref{fig:Fig4}. The additional $^{+19\%}_{-16\%}$ global uncertainty due to the uncertainty in the branching fractions is not included.}
\label{tab:tab7}
\end{table}

\begin{table}[h]
\centering
\begin{tabular}{cc}
$\pt$ range [GeV/$c$] & $\sigma_{\Lb}/\sigma_{\Bd}$ \\
\midrule
0 -- 2 & $0.55\pm0.07$ \\
2 -- 4 & $0.45\pm0.03$ \\
4 -- 6 & $0.51\pm0.02$ \\
6 -- 8 & $0.45\pm0.02$ \\
\hspace{0.2cm}8 -- 10 & $0.43\pm0.02$ \\
10 -- 12 & $0.38\pm0.02$ \\
12 -- 14 & $0.32\pm0.02$ \\
14 -- 16 & $0.31\pm0.02$ \\
16 -- 18 & $0.24\pm0.02$ \\
18 -- 20 & $0.22\pm0.02$ \\
20 -- 22 & $0.22\pm0.02$ \\
22 -- 24 & $0.22\pm0.02$ \\
\end{tabular}
\caption{Ratio of cross-sections for high multiplicity data, as measured using back tracks, shown in red in the right panel of Fig. \ref{fig:Fig4}. The additional $^{+19\%}_{-16\%}$ global uncertainty due to the uncertainty in the branching fractions is not included.}
\label{tab:tab8}
\end{table}

\FloatBarrier
